# Supplementary material for: Resource Allocation to Agents with Restrictions: Maximizing Likelihood with Minimum Compromise
Source: arXiv:2209.05170 source file (2022-09-12)
Supplement: Supplementary file 1 [file appendix.tex]

\begin{figure}
     \includegraphics[scale=0.135]{images/school_vacation.png}
     \includegraphics[scale=0.135]{images/course_classes_heatmap.png}
     \caption{Heatmaps for the School vacation and the Course classes datasets. On large graphs the effect of multiple applications of $HK$ is more noticeable but the baseline is more compatible with the $HK$}
\end{figure}

\begin{figure}
    \includegraphics[scale=0.8]{images/synthetic_and_or.jpg}
    \caption{Comparison between the greedy heuristic and an exhaustive search for both the OR and the AND cases.}
    \includegraphics[scale=0.28]{images/course_classes_relaxation.png}
\end{figure}
